# Supplementary material for: The CGF dark matter fluid
Source: arXiv:2211.02881 ancillary file (2022-11-01)
Supplement: Supplementary file 1 [file CGF_fluid_calculations.pdf]

# Calculations for *The CGF dark matter fluid*

Daniel Friedan

*New High Energy Theory Center and Department of Physics and Astronomy,  
Rutgers, The State University of New Jersey,  
Piscataway, New Jersey 08854-8019 U.S.A. and  
Science Institute, The University of Iceland, Reykjavik, Iceland  
dfriedan@gmail.com      physics.rutgers.edu/~friedan*

November 1, 2022

## ABSTRACT

Details of calculations for *The CGF dark matter fluid*.

## CONTENTS

|    |                                                               |    |
|----|---------------------------------------------------------------|----|
| 1  | Introduction                                                  | 2  |
| 2  | Standard Model action                                         | 2  |
| 3  | SU(2) structure on space-time spinors                         | 3  |
|    | 3.1 Equivalence to a 4-velocity field $u^\alpha(x)$ . . . . . | 3  |
|    | 3.2 A natural SU(2) spin connection . . . . .                 | 3  |
| 4  | Form of the CGF                                               | 5  |
| 5  | Equations of motion                                           | 5  |
| 6  | Solution of the equations of motion                           | 8  |
| 7  | Energy-momentum tensor                                        | 9  |
| 8  | Irrotationality                                               | 13 |
| 9  | Adiabatic time evolution implies a continuity equation        | 13 |
| 10 | Summary of the parametrization                                | 15 |
| 11 | Low density                                                   | 18 |
| 12 | Possibilities of detection and verification?                  | 20 |

## 1 Introduction

Numbers from PDG, NIST ( $c = 1$ , no error bars)

$$\begin{aligned}
\ell_0 &= \frac{\hbar}{m_{\text{Higgs}}} &= 5.2614864632102925 \times 10^{-27} \text{ s} \\
\rho_0 &= \frac{m_{\text{Higgs}}}{\ell_0^3} &= 5.682491786274899 \times 10^{28} \text{ kg/m}^3 \\
\ell &= \frac{1}{\sqrt{G\rho_0}} = \frac{\hbar m_{\text{Planck}}}{m_{\text{Higgs}}^2} &= 15.39389190962883 \text{ cm} \\
M_\ell &= \frac{\ell}{G} = \ell^3 \rho_0 &= 1.042510314426683 \times 10^{-4} \text{ M}_\odot \\
\omega_0 &= \frac{\ell}{\ell_0} = \frac{m_{\text{Planck}}}{m_{\text{Higgs}}} &= 0.9759312573158477 \times 10^{17} \\
g^2 &= \frac{4\pi\alpha}{\sin^2 \theta_W} &= 0.4111966909854108 \\
\lambda^2 &= \frac{g^2}{4} \frac{m_{\text{Higgs}}^2}{m_W^2} &= 0.2490112919526795
\end{aligned} \tag{1.1}$$

$$[G] = \frac{\text{Jm}}{\text{kg}^2} \quad [\rho] = \frac{\text{kg}}{\text{m}^3} \quad \left[ (G\rho)^{-\frac{1}{2}} c \right] = \text{m} \quad \left[ (G\rho)^{-\frac{1}{2}} G^{-1} c^3 \right] = \text{kg} \tag{1.2}$$

$$\begin{aligned}
G &= 6.67430 \times 10^{-11} \text{ m}^3 \text{ kg}^{-1} \text{ s}^{-2} \\
c &= 2.99792458 \times 10^8 \text{ m/s} \\
\hbar &= 1.054571817 \times 10^{-34} \text{ Js} \\
1 \text{ eV} &= 1.602176634 \times 10^{-19} \text{ J} \\
\text{M}_\odot &= 1.988409870698051 \times 10^{30} \text{ kg} \\
H_0 &= 67.4 \text{ (km/s)/Mpc} = 2.184 \times 10^{-18} \text{ s}^{-1} \\
\rho_c &= \frac{3H_0^2}{8\pi G} = 8.53 \times 10^{-27} \text{ kg/m}^3 \\
\frac{\hbar}{m_{\text{Planck}}} &= \sqrt{G\hbar} = 5.391247 \times 10^{-44} \text{ s} \\
\alpha &= \frac{e^2}{4\pi} = 1/137.035999139(31) \\
m_W &= 80.379(12) \text{ GeV} \quad m_Z = 91.1876(21) \text{ GeV} \quad m_{\text{Higgs}} = 125.10(14) \text{ GeV} \\
\frac{m_W}{m_Z} &= \cos \theta_W = 0.88147(13) \quad \sin^2 \theta_W = 0.2230106391
\end{aligned} \tag{1.3}$$

## 2 Standard Model action

See numbers above.

### 3 SU(2) structure on space-time spinors

#### 3.1 Equivalence to a 4-velocity field $u^\alpha(x)$

The Dirac algebra

$$\gamma_\mu \gamma_\nu + \gamma_\nu \gamma_\mu = 2g_{\mu\nu} \quad \gamma_5 = \frac{i}{4!} \epsilon^{\mu\nu\rho\sigma} \gamma_\mu \gamma_\nu \gamma_\rho \gamma_\sigma \quad \gamma_5^2 = 1 \quad (3.1)$$

has a standard representation on  $\mathbb{C}^4$ .

$$\gamma_0 = \begin{pmatrix} 0 & 1 \\ -1 & 0 \end{pmatrix} \quad \gamma_i = \begin{pmatrix} 0 & \sigma_i \\ \sigma_i & 0 \end{pmatrix} \quad \gamma_5 = \begin{pmatrix} 1 & 0 \\ 0 & -1 \end{pmatrix} \quad (3.2)$$

$$g_{\mu\nu} = \text{diag}(-1, 1, 1, 1)$$

where  $\sigma_i$  are the  $2 \times 2$  Pauli matrices,

$$\sigma_i \sigma_j = \delta_{ij} + i\epsilon_{ij}^{\phantom{ij}k} \sigma_k \quad \sigma_i^\dagger = \sigma_i \quad (3.3)$$

The chiral spinors are the eigenspace  $\gamma_5 = 1$ . The generators of  $\text{Spin}(1,3)$  are

$$L_{\mu\nu} = \frac{1}{4} [\gamma_\mu, \gamma_\nu] \quad L_{0k} = \begin{pmatrix} \frac{1}{2} \sigma_k & 0 \\ 0 & -\frac{1}{2} \sigma_k \end{pmatrix} \quad L_{jk} = \begin{pmatrix} \frac{1}{4} [\sigma_j, \sigma_k] & 0 \\ 0 & -\frac{1}{4} [\sigma_j, \sigma_k] \end{pmatrix} \quad (3.4)$$

Adjoint with respect to the standard hermitian form on  $\mathbb{C}^4$  are

$$\gamma_0^\dagger = -\gamma_0 \quad \gamma_i^\dagger = \gamma_i \quad L_{0i}^\dagger = L_{0i} \quad L_{ij}^\dagger = -L_{ij} \quad (3.5)$$

The  $L_{ij}$  are generators of  $\text{SU}(2)$ , as are the  $iL_{0k}$ . Associate this  $\text{SU}(2)$  structure with the 4-velocity  $u_0^\mu = (1, 0, 0, 0)$ . The  $\text{Spin}(1,3)$  action then associates to every 4-velocity  $u^\mu$  an  $\text{SU}(2)$  structure on the spinors such that

$$g_{\mu\nu} u^\mu u^\nu = -1 \quad u^0 > 0 \quad P_\beta^\alpha = \delta_\beta^\alpha + u^\alpha u_\beta \quad (3.6)$$

$$u^\alpha \gamma_\alpha^\dagger = -u^\alpha \gamma_\alpha \quad P_\beta^\alpha \gamma_\alpha^\dagger = P_\beta^\alpha \gamma_\alpha$$

$$\gamma_\mu^\dagger = \gamma_\mu + 2u_\mu u^\alpha \gamma_\alpha = -\gamma_\mu + 2P_\mu^\alpha \gamma_\alpha \quad (3.7)$$

$$u^\alpha L_{\alpha\mu}^\dagger = u^\alpha L_{\alpha\mu} \quad P_\alpha^\mu P_\beta^\nu L_{\mu\nu}^\dagger = -P_\alpha^\mu P_\beta^\nu L_{\mu\nu}$$

This identifies the space of  $\text{SU}(2)$  structures with the space of 4-velocities,

$$\text{SL}(2, \mathbb{C}) / \text{SU}(2) = \text{SO}(1,3) / \text{SO}(3) = \{u^\alpha : u^\alpha u_\alpha = -1, u^0 > 0\} \quad (3.8)$$

because the little group  $\text{SU}(2)$  preserves the  $\text{SU}(2)$  structure associated to  $u_0^\mu$ .

#### 3.2 A natural $\text{SU}(2)$ spin connection

The local Dirac matrices  $\gamma_\mu(x)$  act on the spinors at  $x$ , the fiber  $S_x$ . The local Lorentz generators are

$$L_{\mu\nu}(x) = \frac{1}{4} [\gamma_\mu, \gamma_\nu] \quad [L_{\mu\nu}, \gamma_\alpha] = \gamma_\mu g_{\nu\alpha} - \gamma_\nu g_{\mu\alpha} \quad (3.9)$$

The boost operators relative to  $u^\mu(x)$  are

$$L_\mu = u^\alpha L_{\alpha\mu} \quad u^\alpha L_\alpha = 0 \quad L_\mu^\dagger = L_\mu \quad (3.10)$$

In a spin-rest frame,  $u^\mu = (1, 0, 0, 0)$ ,  $g_{\mu\nu} = \text{diag}(-1, 1, 1, 1)$  and the  $\gamma_\mu(x)$  take the form (3.5) giving

$$L_0 = 0 \quad L_i = \begin{pmatrix} \frac{1}{2}\sigma_i & 0 \\ 0 & -\frac{1}{2}\sigma_i \end{pmatrix} \quad (3.11)$$

The local SU(2) generators are the operators  $iL_\nu$  or, equivalently, the operators  $[L_\mu, L_\nu]$ . The  $L_\mu$  satisfy identities that can be derived in a spin-rest frame.

$$\begin{aligned} [L_\nu, \gamma_\sigma] &= u^\mu \gamma_\mu g_{\nu\sigma} - u_\sigma \gamma_\nu \\ L_\mu L_\nu &= \frac{1}{4} P_{\mu\nu} + \frac{1}{2} u^\alpha \epsilon_{\alpha\mu\nu}{}^\sigma \gamma_5 i L_\sigma \end{aligned} \quad (3.12)$$

$$\begin{aligned} [L_\mu, L_\nu] &= u^\rho \epsilon_{\rho\mu\nu}{}^\sigma \gamma_5 i L_\sigma \\ L_{\mu\nu} &= L_\mu u_\nu - L_\nu u_\mu + [L_\mu, L_\nu] \\ \text{tr}(L_\mu) &= 0 \\ \text{tr}(L_\mu L_\nu) &= \frac{1}{2} P_{\mu\nu} \\ \text{tr}([L_\mu, L_\nu] L_\rho) &= \frac{i}{2} u^\alpha \epsilon_{\alpha\mu\nu\rho} \\ \text{tr}(-[L_\mu, L_\nu][L_{\mu'}, L_{\nu'}]) &= \frac{1}{2} (P_{\mu\mu'} P_{\nu\nu'} - P_{\mu\nu'} P_{\nu\mu'}) \end{aligned} \quad (3.13)$$

The traces are over the two-dimensional vector space of chiral spinors  $(S_+)_x$ .

From the above,

$$\begin{aligned} [L^\nu, [L_\mu, L_\nu]] &= L^\nu L_\mu L_\nu - L^\nu L_\nu L_\mu - L_\mu L_\nu L^\nu + L_\nu L_\mu L^\nu \\ &= 2L^\nu (L_\mu L_\nu + L_\nu L_\mu) - 4L^\nu L_\nu L_\mu \\ &= L^\nu P_{\mu\nu} - 3L_\mu \\ &= -2L_\mu \end{aligned} \quad (3.14)$$

Parallel transport of orthonormal frames lifts to parallel transport of spin frames, since SL(1,3) and Spin(1,3) have the same infinitesimal generators. Therefore the metric covariant derivative  $\nabla_\mu$  acts on spinors such that

$$\nabla_\mu \gamma_\nu = 0 \quad (3.15)$$

Its curvature form

$$F_{\mu\nu}^{\text{metric}} = [\nabla_\mu, \nabla_\nu] \quad (3.16)$$

satisfies

$$\begin{aligned} \nabla_\nu (v^\beta \gamma_\beta) &= (\nabla_\nu v^\beta) \gamma_\beta & \nabla_\mu \nabla_\nu (v^\beta \gamma_\beta) &= (\nabla_\mu \nabla_\nu v^\beta) \gamma_\beta \\ [F_{\mu\nu}^{\text{metric}}, v^\beta \gamma_\beta] &= \nabla_{[\mu} \nabla_{\nu]} (v^\beta \gamma_\beta) = R^\beta{}_{\alpha\mu\nu} v^\alpha \gamma_\beta = R^\alpha{}_{\beta\mu\nu} v^\beta \gamma_\alpha \\ [F_{\mu\nu}^{\text{metric}}, \gamma_\beta] &= R^\alpha{}_{\beta\mu\nu} \gamma_\alpha \end{aligned} \quad (3.17)$$

which has a unique solution since only the identity matrix commutes with all the  $\gamma_\beta$  and  $\nabla_\mu$  is an SO(1,3) connection on the spinor bundle.

$$F_{\mu\nu}^{\text{metric}} = \frac{1}{2} R^{\alpha\beta}{}_{\mu\nu} L_{\alpha\beta} \quad (3.18)$$

The symplectic structure on  $S_x$  depends only on the space-time metric, but the positive hermitian form on  $S_x$  depends on both the metric and on the 4-velocity. The metric connection does not preserve the hermitian structure.

$$\nabla_\mu \gamma_\nu^\dagger = \nabla_\mu (\gamma_\nu + 2u_\nu u^\alpha \gamma_\alpha) = 2\nabla_\mu (u_\nu u^\alpha) \gamma_\alpha \neq 0 \quad (3.19)$$

The modified covariant derivative

$$D_\mu^0 = \nabla_\mu - \nabla_\mu u^\sigma L_\sigma \quad (3.20)$$

It is a natural  $\text{SO}(1,3)$  connection.

$$\begin{aligned} \nabla_\mu L_\nu &= \nabla_\mu u^\alpha L_{\alpha\nu} \\ D_\mu^0 L_\nu &= \nabla_\mu L_\nu - \nabla_\mu u^\sigma [L_\sigma, L_\nu] \\ &= \nabla_\mu u^\alpha L_{\alpha\beta} - \nabla_\mu u^\sigma (L_{\sigma\nu} - L_\sigma u_\nu + L_\nu u_\sigma) \\ &= \nabla_\mu u^\sigma u_\nu L_\sigma \end{aligned} \quad (3.21)$$

so  $D_\mu^0$  preserves the hermitian structure,

$$D_\mu^0 (L_\nu^\dagger) = (D_\mu^0 L_\nu)^\dagger \quad (3.22)$$

so  $D_\mu^0$  is an  $\text{SU}(2)$  connection. Its curvature form is

$$\begin{aligned} F_{\mu\nu}^0 &= [D_\mu^0, D_\nu^0] = [\nabla_\mu - \nabla_\mu u^\alpha L_\alpha, \nabla_\nu - \nabla_\nu u^\beta L_\beta] \\ &= F_{\mu\nu}^{\text{metric}} - (\nabla_\mu \nabla_\nu - \nabla_\nu \nabla_\mu) u^\beta L_\beta - \nabla_\nu u^\beta \nabla_\mu L_\beta + \nabla_\mu u^\beta \nabla_\nu L_\beta \\ &\quad + \nabla_\mu u^\alpha \nabla_\nu u^\beta [L_\alpha, L_\beta] \\ &= \frac{1}{2} R^{\alpha\beta}{}_{\mu\nu} L_{\alpha\beta} - R^\beta{}_{\alpha\mu\nu} u^\alpha L_\beta - \nabla_\nu u^\beta \nabla_\mu u^\alpha L_{\alpha\beta} + \nabla_\mu u^\beta \nabla_\nu u^\alpha L_{\alpha\beta} \\ &\quad + \nabla_\mu u^\alpha \nabla_\nu u^\beta [L_\alpha, L_\beta] \\ &= \left( \frac{1}{2} R^{\alpha\beta}{}_{\mu\nu} - \nabla_\nu u^\beta \nabla_\mu u^\alpha + \nabla_\mu u^\beta \nabla_\nu u^\alpha \right) ([L_\alpha, L_\beta] + L_\alpha u_\beta - L_\beta u_\alpha) \\ &\quad - R^\beta{}_{\alpha\mu\nu} u^\alpha L_\beta + \nabla_\mu u^\alpha \nabla_\nu u^\beta [L_\alpha, L_\beta] \\ &= \left( \frac{1}{2} R^{\alpha\beta}{}_{\mu\nu} - \nabla_\mu u^\alpha \nabla_\nu u^\beta \right) [L_\alpha, L_\beta] \end{aligned} \quad (3.23)$$

## 4 Form of the CGF

## 5 Equations of motion

**Scalar field equations of motion** The scalar field action written in terms of the dimensionless scalar field  $\hat{\phi}$ ,

$$\phi = \frac{v}{\sqrt{2}} \hat{\phi} \quad (5.1)$$

is

$$\begin{aligned}
\frac{1}{\hbar} S_{\text{scalar}} &= \int \left[ \ell^{-2} D_\mu \phi^\dagger D^\mu \phi + \frac{1}{2} \lambda^2 \left( \phi^\dagger \phi - \frac{1}{2} v^2 \right)^2 \right] \ell^4 \sqrt{-g} d^4 x \\
&= \int \frac{1}{\lambda^2} \left[ \ell^{-2} \frac{\lambda^2 v^2}{2} D_\mu \hat{\phi}^\dagger D^\mu \hat{\phi} + \frac{\lambda^4 v^4}{8} \left( \hat{\phi}^\dagger \hat{\phi} - 1 \right)^2 \right] \ell^4 \sqrt{-g} d^4 x \\
&= \int \frac{1}{\lambda^2} \left[ \frac{\ell^{-2} \ell_0^{-2}}{2} D_\mu \hat{\phi}^\dagger D^\mu \hat{\phi} + \frac{\ell_0^{-4}}{8} \left( \hat{\phi}^\dagger \hat{\phi} - 1 \right)^2 \right] \ell^4 \sqrt{-g} d^4 x \\
&= \int \frac{1}{\lambda^2} \left[ \frac{1}{2\omega_0^2} D_\mu \hat{\phi}^\dagger D^\mu \hat{\phi} + \frac{1}{8} \left( \hat{\phi}^\dagger \hat{\phi} - 1 \right)^2 \right] \omega_0^4 \sqrt{-g} d^4 x
\end{aligned} \tag{5.2}$$

and

$$\begin{aligned}
D_\mu \hat{\phi}^\dagger D^\mu \hat{\phi} &= (D_\mu^0 + B_\mu) \hat{\phi}^\dagger (D^{0\mu} + B^\mu) \hat{\phi} \\
&= D_\mu^0 \hat{\phi}^\dagger D^{0\mu} \hat{\phi} - \hat{\phi}^\dagger B_\mu D^{0\mu} \hat{\phi} + D_\mu^0 \hat{\phi}^\dagger B^\mu \hat{\phi} - \hat{\phi}^\dagger B_\mu B^\mu \hat{\phi}
\end{aligned} \tag{5.3}$$

but  $B_\mu B^\mu$  is a multiple of the identity,

$$B_\mu B^\mu = g^{\mu\nu} B_\mu^\sigma B_\nu^\tau L_\sigma L_\tau = g^{\mu\nu} B_\mu^\sigma B_\nu^\tau \frac{1}{4} P_{\sigma\tau} \tag{5.4}$$

so

$$B_\mu B^\mu = \frac{1}{2} \text{tr}(B_\mu B^\mu) \tag{5.5}$$

$$D_\mu \hat{\phi}^\dagger D^\mu \hat{\phi} = D_\mu^0 \hat{\phi}^\dagger D^{0\mu} \hat{\phi} + \text{tr} \left[ B^\mu (\hat{\phi} D_\mu^0 \hat{\phi}^\dagger - \hat{\phi}^\dagger D_\mu^0 \hat{\phi}) \right] - \frac{1}{2} \hat{\phi}^\dagger \hat{\phi} \text{tr}(B_\mu B^\mu) \tag{5.6}$$

Assume  $\hat{\phi}(x)$  is smooth and  $B_\mu = O(\omega_0)$ . Then to leading order in  $\omega_0$

$$\frac{1}{2\omega_0^2} D_\mu \hat{\phi}^\dagger D^\mu \hat{\phi} = -\frac{1}{4} \hat{\phi}^\dagger \hat{\phi} \text{tr} \left( \frac{B_\mu B^\mu}{\omega_0^2} \right) \tag{5.7}$$

$$\frac{1}{\hbar} S_{\text{scalar}} = \int \frac{1}{\lambda^2} \left[ \frac{1}{4} \hat{\phi}^\dagger \hat{\phi} \text{tr} \left( -\frac{B_\mu B^\mu}{\omega_0^2} \right) + \frac{1}{8} \left( \hat{\phi}^\dagger \hat{\phi} - 1 \right)^2 \right] \omega_0^4 \sqrt{-g} d^4 x \tag{5.8}$$

For the CGF,

$$B_\mu = \omega_0 b_0 i L_\mu$$

$$\text{tr} \left( -\frac{B_\mu B^\mu}{\omega_0^2} \right) = \text{tr} (L^\mu L_\mu) b_0^2 = \frac{3}{2} b_0^2 \tag{5.9}$$

$$\begin{aligned}
\frac{1}{\hbar} S_{\text{scalar}} &= \int \frac{1}{\lambda^2} \left[ \frac{1}{4} \hat{\phi}^\dagger \hat{\phi} \frac{3}{2} b_0^2 + \frac{1}{8} \left( \hat{\phi}^\dagger \hat{\phi} - 1 \right)^2 \right] \omega_0^4 \sqrt{-g} d^4 x \\
&= \int \frac{1}{8\lambda^2} \left[ (\hat{\phi}^\dagger \hat{\phi})^2 + 3 \left( b_0^2 - \frac{2}{3} \right) \hat{\phi}^\dagger \hat{\phi} + 1 \right] \omega_0^4 \sqrt{-g} d^4 x
\end{aligned} \tag{5.10}$$

with equation of motion

$$\begin{aligned}
\left[ 2\hat{\phi}^\dagger \hat{\phi} + 3 \left( b_0^2 - \frac{2}{3} \right) \right] \phi &= 0 \\
\phi = 0 \quad \langle b_0^2 \rangle &\geq \frac{2}{3} \\
\hat{\phi}^\dagger \hat{\phi} = 1 - \frac{3}{2} \langle b_0^2 \rangle \quad \langle b_0^2 \rangle &\leq \frac{2}{3}
\end{aligned} \tag{5.11}$$

**Gauge field equations of motion** Vary the gauge action and the leading order scalar action wrt the gauge field.

$$\frac{1}{\hbar} S_{\text{gauge}} = \int \frac{1}{2g^2} \text{tr} (-\ell^{-4} F_{\mu\nu} F^{\mu\nu}) \ell^4 \sqrt{-g} d^4x \quad (5.12)$$

$$\frac{1}{\hbar} S_{\text{scalar}} = \int \frac{1}{8\lambda^2} \left[ 2\hat{\phi}^\dagger \hat{\phi} \text{tr} \left( -\frac{B_\mu B^\mu}{\omega_0^2} \right) + (\hat{\phi}^\dagger \hat{\phi} - 1)^2 \right] \omega_0^4 \sqrt{-g} d^4x$$

$$\delta F_{\mu\nu} = D_\mu \delta B_\nu - D_\nu \delta B_\mu \quad (5.13)$$

$$\delta S_{\text{gauge}} = \hbar \int \frac{2}{g^2} \text{tr} (-\delta B^\mu D^\nu F_{\mu\nu}) \sqrt{-g} d^4x$$

$$\delta S_{\text{scalar}} = \hbar \int \frac{\omega_0^2}{2\lambda^2} \hat{\phi}^\dagger \hat{\phi} \text{tr} (-\delta B^\mu B_\mu) \sqrt{-g} d^4x \quad (5.14)$$

$$\delta S_{\text{gauge}} + \delta S_{\text{scalar}} = \hbar \int \frac{2}{g^2} \text{tr} \left[ -\frac{\delta B^\mu}{\omega_0} \left( \frac{D^\nu F_{\mu\nu}}{\omega_0^3} + \frac{\omega_0^2 g^2 \hat{\phi}^\dagger \hat{\phi} B_\mu}{4\lambda^2 \omega_0} \right) \right] \omega_0^4 \sqrt{-g} d^4x$$

so the leading order gauge field equation of motion is

$$0 = \frac{D^\nu F_{\mu\nu}}{\omega_0^3} + \frac{\omega_0^2 g^2 \hat{\phi}^\dagger \hat{\phi} B_\mu}{4\lambda^2 \omega_0} \quad (5.15)$$

For the CGF,

$$B_\mu = ibL_\mu \quad b = \omega_0 b_0(\zeta) \quad \zeta = \omega_0 T(x) \quad (5.16)$$

The curvature form is

$$\begin{aligned} F_{\mu\nu} &= [D_\mu, D_\nu] = [D_\mu^0 + ibL_\mu, D_\nu^0 + ibL_\nu] \\ &= F_{\mu\nu}^0 + ib([D_\mu^0, L_\nu] - [D_\nu^0, L_\mu]) + i\partial_\mu b L_\nu - i\partial_\nu b L_\mu - b^2 [L_\mu, L_\nu] \\ &= \omega_0^2 (i\omega_0^{-1} \partial_\mu b_0 L_\nu - i\omega_0^{-1} \partial_\nu b_0 L_\mu - b_0^2 [L_\mu, L_\nu]) + O(\omega_0) \\ &= \omega_0^2 \left( i \frac{db_0}{d\zeta} \partial_{[\mu} T L_{\nu]} - b_0^2 [L_\mu, L_\nu] \right) + O(\omega_0) \end{aligned} \quad (5.17)$$

$$\frac{1}{\omega_0^2} F_{\mu\nu} = \frac{db_0}{d\zeta} \partial_{[\mu} T i L_{\nu]} - b_0^2 [L_\mu, L_\nu] + O(\omega_0^{-1})$$

$$b'_0 = \frac{db_0}{d\zeta} \quad b''_0 = \frac{d^2 b_0}{d\zeta^2} \quad (5.18)$$

$$\begin{aligned} \omega_0^{-3} D^\nu F_{\mu\nu} &= ib''_0 \partial^\nu T \partial_{[\mu} T L_{\nu]} \\ &\quad - 2b_0 b'_0 \partial^\nu T [L_\mu, L_\nu] + ib_0 [L^\nu, ib'_0 \partial_{[\mu} T L_{\nu]} - b_0^2 [L_\mu, L_\nu]] \\ &= ib''_0 (\partial^\nu T \partial_\mu T L_\nu - \partial^\nu T \partial_\nu T L_\mu) \\ &\quad - 2b_0 b'_0 \partial^\nu T [L_\mu, L_\nu] + b_0 b'_0 [L^\nu, \partial_\nu T L_\mu] - ib_0^3 [L^\nu, [L_\mu, L_\nu]] \end{aligned} \quad (5.19)$$

Identity (3.14) gives

$$\begin{aligned} \omega_0^{-3} D^\nu F_{\mu\nu} &= -b''_0 \partial^\nu T \partial_\nu T i L_\mu + b''_0 \partial_\mu T \partial^\nu T i L_\nu - 3b_0 b'_0 \partial^\nu T [L_\mu, L_\nu] + 2b_0^3 i L_\mu \\ &= (-b''_0 \partial^\nu T \partial_\nu T + 2b_0^3) i L_\mu + b''_0 \partial_\mu T \partial^\nu T i L_\nu - 3b_0 b'_0 \partial^\nu T [L_\mu, L_\nu] \end{aligned} \quad (5.20)$$

The equation of motion is

$$0 = \left( -\partial^\nu T \partial_\nu T b_0'' + \frac{g^2 \hat{\phi}^\dagger \hat{\phi}}{4\lambda^2} b_0 + 2b_0^3 \right) iL_\mu + b_0'' \partial_\mu T \partial^\nu T iL_\nu - 3b_0 b_0' \partial^\nu T [L_\mu, L_\nu] \quad (5.21)$$

Now contract with  $u^\mu$ .

$$0 = b_0'' (u^\mu \partial_\mu T) \partial^\nu T iL_\nu \quad (5.22)$$

But  $b_0''$ ,  $u^\mu \partial_\mu T \neq 0$  so  $\partial^\nu T iL_\nu = 0$  so

$$u_\mu = -a_\ell \partial_\mu T \quad u^\mu \partial_\mu T = \frac{1}{a_\ell} \quad \partial_\nu T \partial^\nu T = -\frac{1}{a_\ell^2} \quad (5.23)$$

The last two summands in (5.21) vanish since  $u^\mu L_\mu = 0$ . The equation of motion becomes

$$0 = \frac{1}{a_\ell^2} \frac{d^2 b_0}{d\zeta^2} + \left( \frac{g^2 \hat{\phi}^\dagger \hat{\phi}}{4\lambda^2} \right) b_0 + 2b_0^3 \quad (5.24)$$

which is an anharmonic oscillator with conserved energy

$$H = \frac{1}{2} \frac{1}{a_\ell^2} \left( \frac{db_0}{d\zeta} \right)^2 + \frac{1}{2} \left( \frac{g^2 \hat{\phi}^\dagger \hat{\phi}}{4\lambda^2} \right) b_0^2 + \frac{1}{2} b_0^4 \quad (5.25)$$

## 6 Solution of the equations of motion

References for elliptic function identities are given in [1].

**The Jacobi Elliptic function**  $\text{cn}(z, k)$

$$\text{cn}(z + 4K, k) = \text{cn}(z, k) \quad \text{cn}'^2 = (1 - \text{cn}^2)(k'^2 + k^2 \text{cn}^2) \quad (6.1)$$

$$f(z, k) = k \text{cn}(z, k)$$

$$\left( \frac{df}{dz} \right)^2 = (k^2 - f^2)(k'^2 + f^2) = k^2(1 - k^2) + (2k^2 - 1)f^2 - f^4 \quad (6.2)$$

$$\left( \frac{df}{dz} \right)^2 + (1 - 2k^2)f^2 + f^4 = k^2(1 - k^2)$$

**The function**  $F(\zeta, k)$

$$F(\zeta, k) = \frac{k \text{cn}(z, k)}{\zeta'} = \frac{f(z, k)}{\zeta'} \quad \zeta = \frac{2\pi}{4K} z \quad \zeta' = \frac{2\pi}{4K} \quad (6.3)$$

$$F(\zeta + 2\pi) = F(\zeta)$$

$$\frac{df}{dz} = \zeta'^2 \frac{dF}{d\zeta}$$

$$\zeta'^4 \left( \frac{dF}{d\zeta} \right)^2 + (1 - 2k^2) \zeta'^2 F^2 + \zeta'^4 F^4 = k^2(1 - k^2) \quad (6.4)$$

$$\frac{1}{2} \left( \frac{dF}{d\zeta} \right)^2 + \frac{(1 - 2k^2)}{2\zeta'^2} F^2 + \frac{1}{2} F^4 = \frac{k^2(1 - k^2)}{2\zeta'^4}$$



The solution

$$b_0(\zeta) = \frac{1}{a_\ell} F(\zeta, k) \quad (6.5)$$

$$\frac{k^2(1-k^2)}{2\zeta'^4} = \frac{1}{2} \left( \frac{dF}{d\zeta} \right)^2 + \frac{(1-2k^2)}{2\zeta'^2} F^2 + \frac{1}{2} F^4$$

$$H = \frac{1}{2a_\ell^2} \left( \frac{db_0}{d\zeta} \right)^2 + \frac{g^2 \hat{\phi}^\dagger \hat{\phi}}{8\lambda^2} b_0^2 + \frac{1}{2} b_0^4 \quad (6.6)$$

$$a_\ell^4 H = \frac{1}{2} \left( \frac{dF}{d\zeta} \right)^2 + \frac{g^2 \hat{\phi}^\dagger \hat{\phi} a_\ell^2}{8\lambda^2} F^2 + \frac{1}{2} F^4$$

$$a_\ell^4 H = \frac{k^2(1-k^2)}{2\zeta'^4} \frac{g^2 \hat{\phi}^\dagger \hat{\phi} a_\ell^2}{8\lambda^2} = \frac{1-2k^2}{2\zeta'^2}$$

$$\hat{\phi}^\dagger \hat{\phi} = \frac{4\lambda^2}{g^2} \frac{1-2k^2}{\zeta'^2 a_\ell^2} \quad (6.7)$$

In the unbroken phase  $\hat{\phi} = 0$

$$k^2 = \frac{1}{2} \quad \frac{1}{8\zeta'^4} = a_\ell^4 H \quad (6.8)$$

Averaging over a period

$$\langle \text{cn}^2 \rangle = \frac{1}{k^2} \left( k^2 - 1 + \frac{E}{K} \right) \quad \langle F^2 \rangle = \frac{1}{\zeta'^2} \left( k^2 - 1 + \frac{E}{K} \right)$$

$$\langle b_0^2 \rangle = \frac{1}{a_\ell^2} \langle F^2 \rangle = \frac{1}{\zeta'^2 a_\ell^2} \left( k^2 - 1 + \frac{E}{K} \right) \quad (6.9)$$

In the broken phase

$$\hat{\phi}^\dagger \hat{\phi} = 1 - \frac{3}{2} \langle b_0^2 \rangle = 1 - \frac{3}{2} \frac{1}{\zeta'^2 a_\ell^2} \left( k^2 - 1 + \frac{E}{K} \right) \quad (6.10)$$

$$1 = \frac{4\lambda^2}{g^2} (1-2k^2) \frac{1}{\zeta'^2 a_\ell^2} + \frac{3}{2} \frac{1}{\zeta'^2 a_\ell^2} \left( k^2 - 1 + \frac{E}{K} \right)$$

$$\zeta'^2 a_\ell^2 = \frac{4\lambda^2}{g^2} (1-2k^2) + \frac{3}{2} \left( k^2 - 1 + \frac{E}{K} \right) \quad (6.11)$$

## 7 Energy-momentum tensor

scalar field energy-momentum tensor

$$\frac{1}{\hbar} T^\phi_\nu = \frac{1}{\ell^2} (D^\mu \phi^\dagger D_\nu \phi + D_\nu \phi^\dagger D^\mu \phi - \delta_\nu^\mu D_\sigma \phi^\dagger D^\sigma \phi) - \delta_\nu^\mu \frac{\lambda^2}{2} \left( \phi^\dagger \phi - \frac{v^2}{2} \right)^2$$

$$= \frac{1}{\ell^2} \frac{1}{\ell_0^2} \frac{1}{2\lambda^2} \left( D^\mu \hat{\phi}^\dagger D_\nu \hat{\phi} + D_\nu \hat{\phi}^\dagger D^\mu \hat{\phi} - \delta_\nu^\mu D_\sigma \hat{\phi}^\dagger D^\sigma \hat{\phi} \right) - \delta_\nu^\mu \frac{1}{\ell_0^4} \frac{1}{8\lambda^2} \left( \hat{\phi}^\dagger \hat{\phi} - 1 \right)^2 \quad (7.1)$$

$$= \frac{1}{\ell_0^4} \frac{1}{8\lambda^2} \left[ \frac{4}{\omega_0^2} \left( D^\mu \hat{\phi}^\dagger D_\nu \hat{\phi} + D_\nu \hat{\phi}^\dagger D^\mu \hat{\phi} - \delta_\nu^\mu D_\sigma \hat{\phi}^\dagger D^\sigma \hat{\phi} \right) - \delta_\nu^\mu \left( \hat{\phi}^\dagger \hat{\phi} - 1 \right)^2 \right]$$

Use

$$B_\mu B_\nu + B_\nu B_\mu = B_\mu^\sigma B_\nu^\tau (L_\sigma L_\tau + L_\tau L_\sigma) = B_\mu^\sigma B_\nu^\tau \frac{1}{2} P_{\sigma\tau} = \text{tr}(B_\mu B_\nu) \quad (7.2)$$

to get

$$\begin{aligned} D_\mu \hat{\phi}^\dagger D_\nu \hat{\phi} &= (D_\mu^0 + B_\mu) \hat{\phi}^\dagger (D_\nu^0 + B_\nu) \hat{\phi} \\ &= D_\mu^0 \hat{\phi}^\dagger D_\nu^0 \hat{\phi} - \hat{\phi}^\dagger B_\mu D_\nu^0 \hat{\phi} + D_\mu^0 \hat{\phi}^\dagger B_\nu \hat{\phi} - \hat{\phi}^\dagger B_\mu B_\nu \hat{\phi} \\ D_\mu \hat{\phi}^\dagger D_\nu \hat{\phi} + D_\nu \hat{\phi}^\dagger D_\mu \hat{\phi} &= \left( D_\mu^0 \hat{\phi}^\dagger D_\nu^0 \hat{\phi} - \hat{\phi}^\dagger B_\mu D_\nu^0 \hat{\phi} + D_\mu^0 \hat{\phi}^\dagger B_\nu \hat{\phi} \right) + \mu \leftrightarrow \nu \\ &\quad - \hat{\phi}^\dagger (B_\mu B_\nu + B_\nu B_\mu) \hat{\phi} \\ &= \left( D_\mu^0 \hat{\phi}^\dagger D_\nu^0 \hat{\phi} - \hat{\phi}^\dagger B_\mu D_\nu^0 \hat{\phi} + D_\mu^0 \hat{\phi}^\dagger B_\nu \hat{\phi} \right) + \mu \leftrightarrow \nu \\ &\quad - \hat{\phi}^\dagger \hat{\phi} \text{tr}(B_\mu B_\nu) \end{aligned} \quad (7.3)$$

so, to leading order,

$$\frac{4}{\omega_0^2} \left( D^\mu \hat{\phi}^\dagger D_\nu \hat{\phi} + D_\nu \hat{\phi}^\dagger D^\mu \hat{\phi} - \delta_\nu^\mu D_\sigma \hat{\phi}^\dagger D^\sigma \hat{\phi} \right) = \hat{\phi}^\dagger \hat{\phi} \text{tr} \frac{2}{\omega_0^2} (-2B^\mu B_\nu + \delta_\nu^\mu B_\sigma B^\sigma) \quad (7.4)$$

$$\frac{1}{\hbar} T_\nu^{\phi\mu} = \frac{1}{\ell_0^4} \frac{1}{8\lambda^2} \left[ \hat{\phi}^\dagger \hat{\phi} \text{tr} \frac{2}{\omega_0^2} (-2B^\mu B_\nu + \delta_\nu^\mu B_\sigma B^\sigma) - \delta_\nu^\mu \left( \hat{\phi}^\dagger \hat{\phi} - 1 \right)^2 \right] \quad (7.5)$$

For the CGF, with  $B_\mu = \omega_0 b_0 i L_\mu$

$$\begin{aligned} \text{tr} \frac{2}{\omega_0^2} (-2B^\mu B_\nu + \delta_\nu^\mu B_\sigma B^\sigma) &= b_0^2 \text{tr} (4L^\mu L_\nu - 2\delta_\nu^\mu L_\sigma L^\sigma) = b_0^2 (2P_\nu^\mu - \delta_\nu^\mu P_\sigma^\sigma) \\ &= b_0^2 (2P_\nu^\mu - 3\delta_\nu^\mu) \end{aligned} \quad (7.6)$$

so

$$\begin{aligned} \frac{1}{\hbar} T_\nu^{\phi\mu} &= \frac{1}{\ell_0^4} \frac{1}{8\lambda^2} \left[ \hat{\phi}^\dagger \hat{\phi} b_0^2 (2P_\nu^\mu - 3\delta_\nu^\mu) - \delta_\nu^\mu \left( \hat{\phi}^\dagger \hat{\phi} - 1 \right)^2 \right] \\ &= \frac{1}{\ell_0^4} \frac{1}{8\lambda^2} \left[ \hat{\phi}^\dagger \hat{\phi} b_0^2 (3u^\mu u_\nu - P_\nu^\mu) + \left( \hat{\phi}^\dagger \hat{\phi} - 1 \right)^2 (u^\mu u_\nu - P_\nu^\mu) \right] \end{aligned} \quad (7.7)$$

**gauge field energy-momentum tensor**

$$\begin{aligned} \frac{1}{\hbar} T_\nu^{\text{gauge}\mu} &= \frac{1}{\ell^4 g^2} \text{tr} \left( -2F^\mu{}_\sigma F_\nu{}^\sigma + \frac{1}{2} \delta_\nu^\mu F_{\rho\sigma} F^{\rho\sigma} \right) \\ &= \frac{1}{\ell_0^4} \frac{2}{g^2} \frac{1}{\omega_0^4} \text{tr} \left( -F^\mu{}_\sigma F_\nu{}^\sigma + \frac{1}{4} \delta_\nu^\mu F_{\rho\sigma} F^{\rho\sigma} \right) \end{aligned} \quad (7.8)$$

$$\frac{1}{\omega_0^2} F_{\mu\nu} = \frac{db_0}{d\zeta} \partial_{[\mu} T i L_{\nu]} - b_0^2 [L_\mu, L_\nu] \quad (7.9)$$

$$\begin{aligned}
\frac{1}{\omega_0^4} \text{tr} (-F_{\mu\sigma} F_\nu^\sigma) &= \text{tr} \left[ - \left( \frac{db_0}{d\zeta} \partial_{[\mu} T i L_{\sigma]} - b_0^2 [L_\mu, L_\sigma] \right) \right. \\
&\quad \left. \left( \frac{db_0}{d\zeta} \partial_{[\nu} T i L^{\sigma]} - b_0^2 [L_\nu, L^\sigma] \right) \right] \\
&= \left( \frac{db_0}{d\zeta} \right)^2 \text{tr} (\partial_{[\mu} T L_{\sigma]} \partial_{[\nu} T L^{\sigma]}) - b_0^4 \text{tr} ([L_\mu, L_\sigma] [L_\nu, L^\sigma]) \\
&= \left( \frac{db_0}{d\zeta} \right)^2 \text{tr} [(\partial_\mu T L_\sigma - \partial_\sigma T L_\mu)(\partial_\nu T L^\sigma - \partial^\sigma T L_\nu)] \\
&\quad + b_0^4 \frac{1}{2} (P_{\mu\nu} g^{\sigma\sigma'} P_{\sigma\sigma'} - g^{\sigma\sigma'} P_{\mu\sigma} P_{\nu\sigma'}) \\
&= \left( \frac{db_0}{d\zeta} \right)^2 \frac{1}{2} [\partial_\mu T \partial_\nu T P_\sigma^\sigma - \partial_\sigma T \partial_\nu T P_\mu^\sigma - \partial_\mu T \partial_\sigma T P_\nu^\sigma \\
&\quad + \partial_\sigma T \partial^\sigma T P_{\mu\nu}] + b_0^4 P_{\mu\nu} \\
&= \left( \frac{db_0}{d\zeta} \right)^2 \frac{1}{2} (3\partial_\mu T \partial_\nu T + \partial_\sigma T \partial^\sigma T P_{\mu\nu}) + b_0^4 P_{\mu\nu} \\
&= \frac{1}{2a_\ell^2} \left( \frac{db_0}{d\zeta} \right)^2 (3u_\mu u_\nu - P_{\mu\nu}) + b_0^4 P_{\mu\nu}
\end{aligned} \tag{7.10}$$

$$\begin{aligned}
\frac{1}{\omega_0^4} \text{tr} \left( -F_{\mu\sigma} F_\nu^\sigma + \frac{1}{4} g_{\mu\nu} F_{\rho\sigma} F^{\rho\sigma} \right) &= \frac{1}{2a_\ell^2} \left( \frac{db_0}{d\zeta} \right)^2 \left( 3u_\mu u_\nu + \frac{3}{4} g_{\mu\nu} - P_{\mu\nu} + \frac{3}{4} g_{\mu\nu} \right) \\
&\quad + b_0^4 \left( P_{\mu\nu} - \frac{3}{4} g_{\mu\nu} \right) \\
&= \frac{1}{2a_\ell^2} \left( \frac{db_0}{d\zeta} \right)^2 \left( 3u_\mu u_\nu + \frac{3}{4} g_{\mu\nu} - P_{\mu\nu} + \frac{3}{4} g_{\mu\nu} \right) \\
&\quad + b_0^4 \left( P_{\mu\nu} - \frac{3}{4} g_{\mu\nu} \right) \\
&= \frac{1}{4a_\ell^2} \left( \frac{db_0}{d\zeta} \right)^2 (6u_\mu u_\nu + 3(-u_\mu u_\nu + P_{\mu\nu}) - 2P_{\mu\nu}) \\
&\quad + b_0^4 \left( P_{\mu\nu} - \frac{3}{4} (-u_\mu u_\nu + P_{\mu\nu}) \right) \\
&= \frac{1}{4} \left[ \frac{1}{a_\ell^2} \left( \frac{db_0}{d\zeta} \right)^2 + b_0^4 \right] (3u_\mu u_\nu + P_{\mu\nu})
\end{aligned} \tag{7.11}$$

$$\begin{aligned}
\frac{1}{\hbar} T_{\nu}^{\text{gauge}\mu} &= \frac{1}{\ell_0^4} \frac{1}{2g^2} \left[ \frac{1}{a_\ell^2} \left( \frac{db_0}{d\zeta} \right)^2 + b_0^4 \right] (3u^\mu u_\nu + P_\nu^\mu) \\
&= \frac{1}{\ell_0^4} \frac{1}{g^2} \left[ H - \frac{g^2 \hat{\phi}^\dagger \hat{\phi}}{8\lambda^2} b_0^2 \right] (3u_\mu u_\nu + P_{\mu\nu})
\end{aligned} \tag{7.12}$$

**combined energy-momentum tensor**

$$\rho_0 = \frac{\hbar}{\ell_0^4} \tag{7.13}$$

$$\begin{aligned}
T_\nu^\mu &= T_{\nu}^{\text{gauge}\mu} + T_{\nu}^{\phi\mu} \\
&= \rho_0 \left[ \left( \frac{1}{g^2} H - \frac{\hat{\phi}^\dagger \hat{\phi}}{8\lambda^2} b_0^2 \right) (3u_\mu u_\nu + P_{\mu\nu}) \right. \\
&\quad \left. + \frac{\hat{\phi}^\dagger \hat{\phi} b_0^2}{8\lambda^2} (3u^\mu u_\nu - P_\nu^\mu) + \frac{1}{8\lambda^2} \left( \hat{\phi}^\dagger \hat{\phi} - 1 \right)^2 (u^\mu u_\nu - P_\nu^\mu) \right] \\
&= \rho_0 \left[ \frac{1}{g^2} H (3u_\mu u_\nu + P_{\mu\nu}) - \frac{\hat{\phi}^\dagger \hat{\phi} b_0^2}{4\lambda^2} P_\nu^\mu + \frac{1}{8\lambda^2} \left( \hat{\phi}^\dagger \hat{\phi} - 1 \right)^2 (u^\mu u_\nu - P_\nu^\mu) \right]
\end{aligned} \tag{7.14}$$

**density and pressure**

$$T_\nu^\mu = \rho u^\mu u_\nu + p P_\nu^\mu \tag{7.15}$$

$$\begin{aligned}
\frac{\rho}{\rho_0} &= \frac{3}{g^2} H + \frac{1}{8\lambda^2} \left( \hat{\phi}^\dagger \hat{\phi} - 1 \right)^2 \\
\frac{p}{\rho_0} &= \frac{1}{g^2} H - \frac{\hat{\phi}^\dagger \hat{\phi} b_0^2}{4\lambda^2} - \frac{1}{8\lambda^2} \left( \hat{\phi}^\dagger \hat{\phi} - 1 \right)^2 \\
&= \frac{1}{g^2} H - \frac{\hat{\phi}^\dagger \hat{\phi} \langle b_0^2 \rangle}{4\lambda^2} - \frac{1}{8\lambda^2} \left( \hat{\phi}^\dagger \hat{\phi} - 1 \right)^2
\end{aligned} \tag{7.16}$$

**in the unbroken phase**

$$\frac{\rho}{\rho_0} = \frac{3}{g^2} H + \frac{1}{8\lambda^2} \quad \frac{p}{\rho_0} = \frac{1}{g^2} H - \frac{1}{8\lambda^2} \tag{7.17}$$

**in the broken phase**

$$\hat{\phi}^\dagger \hat{\phi} = 1 - \frac{3}{2} \langle b_0^2 \rangle \tag{7.18}$$

$$\frac{\rho}{\rho_0} = \frac{3}{g^2} H + \frac{9}{32\lambda^2} \langle b_0^2 \rangle^2 \quad \frac{p}{\rho_0} = \frac{1}{g^2} H - \frac{\hat{\phi}^\dagger \hat{\phi}}{4\lambda^2} \langle b_0^2 \rangle - \frac{9}{32\lambda^2} \langle b_0^2 \rangle^2 \tag{7.19}$$

**equivalence with the cosmological equation of state**

See section 10 below.

## 8 Irrotationality

Consider the first order differential operators

$$S_\mu = P_\mu^\rho \partial_\rho = \partial_\mu + u_\mu u^\rho \partial_\rho \quad (8.1)$$

Calculate the commutators

$$\begin{aligned} [S_\mu, S_\nu] &= [P_\mu^\rho \partial_\rho, P_\nu^\sigma \partial_\sigma] = (P_\mu^\rho \partial_\rho P_\nu^\sigma - P_\nu^\sigma \partial_\sigma P_\mu^\rho) \partial_\sigma \\ &= (P_\mu^\rho \partial_\rho P_\nu^\sigma - P_\nu^\sigma \partial_\sigma P_\mu^\rho) (P_\sigma^\tau - u^\tau u_\sigma) \partial_\tau \end{aligned} \quad (8.2)$$

$$= (P_\mu^\rho \partial_\rho P_\nu^\sigma - P_\nu^\sigma \partial_\sigma P_\mu^\rho) S_\sigma + (P_\mu^\rho \partial_\rho P_\nu^\sigma - P_\nu^\sigma \partial_\sigma P_\mu^\rho) (-u^\tau u_\sigma) \partial_\tau$$

$$[S_\mu, S_\nu] - T_{\mu\nu}^\sigma S_\sigma = A_{\mu\nu} u^\tau \partial_\tau \quad T_{\mu\nu}^\sigma = (P_\mu^\rho \partial_\rho P_\nu^\sigma - P_\nu^\sigma \partial_\sigma P_\mu^\rho) \quad (8.3)$$

$$A_{\mu\nu} = -(P_\mu^\rho \partial_\rho P_\nu^\sigma - P_\nu^\sigma \partial_\sigma P_\mu^\rho) u_\sigma = P_{[\mu}^\rho P_{\nu]}^\sigma \partial_\rho u_\sigma = P_\mu^\rho P_\nu^\sigma \partial_{[\rho} u_{\sigma]} \quad (8.4)$$

By taking a linear frame at  $x$  in which  $u^i = 0$  and  $u_i = 0$  we see that

$$A_{\mu\nu} = 0 \quad \Leftrightarrow \quad u_{[\mu} \partial_\nu u_{\rho]} = 0 \quad (8.5)$$

So  $u^\mu(x)$  irrotational implies that the operators  $S_\mu$  are holonomic,

$$[S_\mu, S_\nu] - T_{\mu\nu}^\sigma S_\sigma = 0 \quad (8.6)$$

which in turn implies that there exists a nonzero holonomic function, i.e. a solution of

$$S_\mu T = \partial_\mu T + u_\mu u^\sigma \partial_\sigma T = 0 \quad (8.7)$$

So irrotationality implies the existence of a time coordinate  $T(x)$ .

## 9 Adiabatic time evolution implies a continuity equation

$$\frac{1}{\omega_0^4} \text{tr}(-F_{\mu\sigma} F_\nu^\sigma) = \frac{1}{2a_\ell^2} \left( \frac{db_0}{d\zeta} \right)^2 (3u_\mu u_\nu - P_{\mu\nu}) + b_0^4 P_{\mu\nu} + O(\omega_0^{-1}) \quad (9.1)$$

$$\frac{1}{\omega_0^4} \text{tr}(-F_{\mu\sigma} F^{\mu\sigma}) = -\frac{3}{a_\ell^2} \left( \frac{db_0}{d\zeta} \right)^2 + 3b_0^4 + O(\omega_0^{-1})$$

$$\begin{aligned} \frac{1}{\hbar} S_{\text{gauge}} &= \int \frac{1}{2g^2} \text{tr}(-F_{\mu\nu} F^{\mu\nu}) \sqrt{-g} d^4x \\ &= \int \frac{3\omega_0^4}{2g^2} \left[ -\frac{1}{a_\ell^2} \left( \frac{db_0}{d\zeta} \right)^2 + b_0^4 \right] \sqrt{-g} d^4x + O(\omega_0^3) \end{aligned} \quad (9.2)$$

$$\frac{1}{\hbar} S_{\text{scalar}} = \int \frac{\omega_0^4}{8\lambda^2} \left[ 3\hat{\phi}^\dagger \hat{\phi} b_0^2 + (\hat{\phi}^\dagger \hat{\phi} - 1)^2 \right] \sqrt{-g} d^4x + O(\omega_0^3) \quad (9.3)$$

In the CGF rest frame,

$$\begin{aligned} ds^2 &= \ell^2 g_{\mu\nu} dx^\mu dx^\nu \quad g_{\mu\nu} dx^\mu dx^\nu = a_\ell(x)^2 \left[ -(dT)^2 + g_{ij}^{(3)}(x) dx^i dx^j \right] \\ \sqrt{-g} &= a_\ell^4 \sqrt{\det g_{ij}^{(3)}} \quad d^4x = dT d^3x = \frac{d\zeta d^3x}{\omega_0} \quad \zeta = \omega_0 T \end{aligned} \quad (9.4)$$

and

$$b_0(\zeta) = \frac{1}{a_\ell} F(\zeta, k) \quad (9.5)$$

$$\begin{aligned} \frac{1}{\hbar} S_{\text{CGF}} &= \int \frac{3\omega_0^4}{g^2} \left[ -\frac{1}{2a_\ell^2} \left( \frac{db_0}{d\zeta} \right)^2 + \frac{g^2 \hat{\phi}^\dagger \hat{\phi}}{8\lambda^2} b_0^2 + \frac{b_0^4}{2} + \frac{g^2 (\hat{\phi}^\dagger \hat{\phi} - 1)^2}{24\lambda^2} \right] \sqrt{-g} d^4x \\ &= \int \frac{3\omega_0^4}{g^2} \left[ -\frac{1}{2} \left( \frac{dF}{d\zeta} \right)^2 + \frac{g^2 \hat{\phi}^\dagger \hat{\phi} a_\ell^2}{8\lambda^2} F^2 + \frac{1}{2} F^4 + \frac{g^2 (\hat{\phi}^\dagger \hat{\phi} - 1)^2 a_\ell^4}{24\lambda^2} \right] \frac{\sqrt{-g}}{a_\ell^4} d^4x \end{aligned} \quad (9.6)$$

$$\begin{aligned} \frac{1}{\hbar} S_{\text{CGF}} &= \\ \int d\zeta \int d^3x \sqrt{\det g_{ij}^{(3)}} \frac{3\omega_0^3}{g^2} &\left[ -\frac{1}{2} \left( \frac{dF}{d\zeta} \right)^2 + \frac{g^2 \hat{\phi}^\dagger \hat{\phi} a_\ell^2}{8\lambda^2} F^2 + \frac{1}{2} F^4 + \frac{g^2 (\hat{\phi}^\dagger \hat{\phi} - 1)^2 a_\ell^4}{24\lambda^2} \right] \end{aligned} \quad (9.7)$$

At leading order in  $\omega_0$  each small volume element  $d^3x$  of the fluid is an independent anharmonic oscillator decoupled from the rest of the fluid (ultralocality). The coupling constants of each anharmonic oscillator vary slowly in time compared to the period of oscillation. In such an adiabatic time evolution, the adiabatic invariant  $\oint pdq$  stays constant in time, where  $q$  is the oscillator degree of freedom,  $p$  its canonical conjugate, and the integral is over one period of oscillation. Measured in quanta, the adiabatic invariant is

$$\frac{1}{2\pi\hbar} \oint pdq = \frac{1}{2\pi\hbar} \int_0^{2\pi} p \frac{dq}{d\zeta} d\zeta \quad (9.8)$$

Taking  $q = F$ ,

$$\frac{1}{\hbar} p = d^3x \sqrt{\det g_{ij}^{(3)}} \frac{3\omega_0^3}{g^2} \frac{dF}{d\zeta} \quad (9.9)$$

$$\frac{1}{2\pi\hbar} \oint pdq = d^3x \sqrt{\det g_{ij}^{(3)}} N(x) \quad (9.10)$$

$$N(x) = \frac{3\omega_0^3}{g^2} \frac{1}{2\pi} \int_0^{2\pi} \left( \frac{dF}{d\zeta} \right)^2 d\zeta$$

and

$$\begin{aligned} \frac{1}{2\pi} \int_0^{2\pi} \left( \frac{dF}{d\zeta} \right)^2 d\zeta &= \frac{1}{2\pi} \int_0^{4K} \frac{1}{\zeta'^2} \frac{k^2}{\zeta'^2} \left( \frac{d \operatorname{cn}}{dz} \right)^2 \zeta' dz \\ &= \frac{1}{2\pi \zeta'^3} \int_0^{4K} k^2 \left( \frac{d \operatorname{cn}}{dz} \right)^2 dz \\ &= \frac{1}{K \zeta'^2} \frac{1}{3} [(1 - k^2)K + (2k^2 - 1)E] \\ &= \frac{1}{3 \zeta'^2} \left[ 1 - k^2 + (2k^2 - 1) \frac{E}{K} \right] \end{aligned} \quad (9.11)$$

so

$$\begin{aligned} N(x) &= \frac{3\omega_0^3}{g^2} \frac{1}{2\pi} \int_0^{2\pi} \left( \frac{dF}{d\zeta} \right)^2 d\zeta \\ &= \frac{\omega_0^3}{g^2 \zeta'^2} \left[ 1 - k^2 + (2k^2 - 1) \frac{E}{K} \right] \end{aligned} \quad (9.12)$$

and the adiabatic invariance condition is

$$0 = \frac{\partial}{\partial T} \left[ \sqrt{\det g_{ij}^{(3)}} N(x) \right] = \frac{\partial}{\partial T} \left[ \frac{\sqrt{-g}}{a_\ell^4} a_\ell u^0 N(x) \right] = \partial_\mu \left[ \frac{N(x)}{\ell^3 a_\ell^3} \ell^3 u^\mu \sqrt{-g} \right] \quad (9.13)$$

which is the continuity equation for the number density

$$n(x) = \frac{N(x)}{(\ell a_\ell)^3} \quad (9.14)$$

$$\partial_\mu J^\mu = 0 \quad J^\mu(x) = n(x) \ell^3 u^\mu(x) \sqrt{-g} d^4 x \quad (9.15)$$

## 10 Summary of the parametrization

$$C_1 = \frac{1}{2} k^2 (1 - k^2) \quad C_2 = 1 - 2k^2$$

$$C_3 = k^2 - 1 + \frac{E}{K} \quad C_4 = \zeta' \left[ 1 - k^2 + (2k^2 - 1) \frac{E}{K} \right] \quad \zeta' = \frac{2\pi}{4K} \quad (10.1)$$

$$\hat{a} = \zeta' a_\ell$$

$$H = \frac{k^2(1 - k^2)}{2\zeta'^4 a_\ell^4} = \frac{C_1}{\hat{a}^4}$$

$$\frac{g^2 \hat{\phi}^\dagger \hat{\phi}}{4\lambda^2} = \frac{1 - 2k^2}{\zeta'^2 a_\ell^2} = \frac{C_2}{\hat{a}^2} \quad (10.2)$$

$$\hat{\phi}^\dagger \hat{\phi} = \frac{4\lambda^2 C_2}{g^2 \hat{a}^2}$$

$$\langle b_0^2 \rangle = \left( k^2 - 1 + \frac{E}{K} \right) \frac{1}{\zeta'^2 a_\ell^2} = \frac{C_3}{\hat{a}^2}$$

$$\begin{aligned} \frac{\rho}{\rho_0} &= \frac{3}{g^2} H + \frac{1}{8\lambda^2} \left( \hat{\phi}^\dagger \hat{\phi} - 1 \right)^2 \\ &= \frac{3}{g^2} \frac{C_1}{\hat{a}^4} + \frac{1}{8\lambda^2} \left( \frac{4\lambda^2 C_2}{g^2 \hat{a}^2} - 1 \right)^2 \\ \frac{p}{\rho_0} &= \frac{1}{g^2} H - \frac{1}{4\lambda^2} \hat{\phi}^\dagger \hat{\phi} \langle b_0^2 \rangle - \frac{1}{8\lambda^2} \left( \hat{\phi}^\dagger \hat{\phi} - 1 \right)^2 \\ &= \frac{1}{g^2} \frac{C_1}{\hat{a}^4} - \frac{1}{4\lambda^2} \frac{4\lambda^2 C_2}{g^2 \hat{a}^2} \frac{C_3}{\hat{a}^2} - \frac{1}{8\lambda^2} \left( \frac{4\lambda^2 C_2}{g^2 \hat{a}^2} - 1 \right)^2 \\ &= \frac{1}{g^2} \frac{1}{\hat{a}^4} (C_1 - C_2 C_3) - \frac{1}{8\lambda^2} \left( \frac{4\lambda^2 C_2}{g^2 \hat{a}^2} - 1 \right)^2 \end{aligned} \quad (10.3)$$

$$\begin{aligned} \ell_0^3 n &= \frac{1}{a_\ell^3} \frac{1}{g^2 \zeta'^2} \left[ 1 - k^2 + (2k^2 - 1) \frac{E}{K} \right] \\ &= \frac{1}{\hat{a}^3} \frac{1}{g^2} C_4 \end{aligned}$$

unbroken phase

$$k^2 = \frac{1}{2} \quad C_1 = \frac{1}{8} \quad C_2 = 0 \quad C_3 = -\frac{1}{2} + \frac{E}{K} \quad C_4 = \frac{1}{2}\zeta' \quad \zeta' = \frac{2\pi}{4K} \quad (10.4)$$

$$\langle b_0^2 \rangle = \frac{C_3}{\hat{a}^2} \geq \frac{2}{3} \quad \hat{a}^2 \leq \frac{3}{2}C_3 \quad (10.5)$$

$$\begin{aligned} \frac{\rho}{\rho_0} &= \frac{1}{\hat{a}^4} \frac{3}{8g^2} + \frac{1}{8\lambda^2} \\ \frac{p}{\rho_0} &= \frac{1}{\hat{a}^4} \frac{1}{8g^2} - \frac{1}{8\lambda^2} \end{aligned} \quad (10.6)$$

$$\ell_0^3 n = \frac{1}{\hat{a}^3} \frac{1}{g^2} C_4$$

broken phase

$$\begin{aligned} \hat{\phi}^\dagger \hat{\phi} &= 1 - \frac{3}{2} \langle b_0^2 \rangle \quad \hat{\phi}^\dagger \hat{\phi} + \frac{3}{2} \langle b_0^2 \rangle = 1 \quad \frac{4\lambda^2}{g^2} \frac{C_2}{\hat{a}^2} + \frac{3}{2} \frac{C_3}{\hat{a}^2} = 1 \\ \hat{a}^2 &= \frac{4\lambda^2}{g^2} C_2 + \frac{3}{2} C_3 \end{aligned} \quad (10.7)$$

$$\begin{aligned} \frac{\rho}{\rho_0} &= \frac{1}{\hat{a}^4} \left( \frac{3}{g^2} C_1 + \frac{9}{32\lambda^2} C_3^2 \right) \\ \frac{p}{\rho_0} &= \frac{1}{\hat{a}^4} \left[ \frac{1}{g^2} (C_1 - C_2 C_3) - \frac{9}{32\lambda^2} C_3^2 \right] \\ \ell_0^3 n &= \frac{1}{\hat{a}^3} \frac{1}{g^2} C_4 \end{aligned} \quad (10.8)$$

Comparison with CGF cosmological construction

unbroken phase (cosmology on left, fluid on right)

$$t_{\text{Higgs}} = \ell_0 \quad (10.9)$$

|                                                                                                                                 |                                                                                                          |
|---------------------------------------------------------------------------------------------------------------------------------|----------------------------------------------------------------------------------------------------------|
| $\rho_{\text{CGF}} = \frac{\hbar}{t_{\text{Higgs}}^4} \left( \frac{3}{8g^2} \frac{1}{\hat{a}^4} + \frac{1}{8\lambda^2} \right)$ | $\rho = \frac{\hbar}{\ell_0^4} \left( \frac{3}{8g^2} \frac{1}{\hat{a}^4} + \frac{1}{8\lambda^2} \right)$ |
| $p_{\text{CGF}} = \frac{\hbar}{t_{\text{Higgs}}^4} \left( \frac{1}{8g^2} \frac{1}{\hat{a}^4} - \frac{1}{8\lambda^2} \right)$    | $p = \frac{\hbar}{\ell_0^4} \left( \frac{1}{8g^2} \frac{1}{\hat{a}^4} - \frac{1}{8\lambda^2} \right)$    |



broken phase

|                                                                                                                |                                                                                                     |
|----------------------------------------------------------------------------------------------------------------|-----------------------------------------------------------------------------------------------------|
| $\alpha^2 \langle b^2 \rangle = k^2 - 1 + \frac{E}{K}$                                                         | $\hat{a}^2 \langle b_0^2 \rangle = k^2 - 1 + \frac{E}{K}$                                           |
| $\alpha^2 \mu^2 = 1 - 2k^2$                                                                                    | $\hat{a}^2 \frac{g^2 \hat{\phi}^\dagger \hat{\phi}}{4\lambda^2} = 1 - 2k^2$                         |
| $\alpha^4 E_{\text{CGF}} = \frac{k^2(1 - k^2)}{2}$                                                             | $\hat{a}^4 H = \frac{k^2(1 - k^2)}{2}$                                                              |
| $\alpha^2 \hat{a}^2 = \frac{3}{2} \alpha^2 \langle b^2 \rangle + \frac{4\lambda^2}{g^2} (1 - 2k^2)$            | $\hat{a}^2 = \frac{3}{2} \hat{a}^2 \langle b_0^2 \rangle + \frac{4\lambda^2}{g^2} (1 - 2k^2)$       |
| $\frac{2(\phi^\dagger \phi)_0}{v^2} = 1 - \frac{3}{2} \frac{\alpha^2 \langle b^2 \rangle}{\alpha^2 \hat{a}^2}$ | $\hat{\phi}^\dagger \hat{\phi} = 1 - \frac{3}{2} \frac{\hat{a}^2 \langle b_0^2 \rangle}{\hat{a}^2}$ |

|                                                                                                                                                                                                     |                                                                                                                                                                                 |
|-----------------------------------------------------------------------------------------------------------------------------------------------------------------------------------------------------|---------------------------------------------------------------------------------------------------------------------------------------------------------------------------------|
| $\hat{\rho}_{\text{CGF}} = \frac{3}{g^2} \frac{E_{\text{CGF}}}{\hat{a}^4} + \frac{9}{32\lambda^2} \frac{\langle b^2 \rangle^2}{\hat{a}^4}$                                                          | $\frac{\rho}{\rho_0} = \frac{3}{g^2} H + \frac{9}{32\lambda^2} \langle b_0^2 \rangle^2$                                                                                         |
| $\hat{p}_{\text{CGF}} = \frac{1}{g^2} \frac{E_{\text{CGF}}}{\hat{a}^4} - \frac{1}{g^2} \frac{\mu^2 \langle b^2 \rangle}{\hat{a}^4} - \frac{9}{32\lambda^2} \frac{\langle b^2 \rangle^2}{\hat{a}^4}$ | $\frac{p}{\rho_0} = \frac{1}{g^2} H - \frac{1}{g^2} \frac{g^2 \hat{\phi}^\dagger \hat{\phi}}{4\lambda^2} \langle b_0^2 \rangle - \frac{9}{32\lambda^2} \langle b_0^2 \rangle^2$ |

|                                                                        |                                                                              |
|------------------------------------------------------------------------|------------------------------------------------------------------------------|
| $\frac{K_{\text{EW}}}{2K} \alpha^3 = 1 - k^2 + (2k^2 - 1) \frac{E}{K}$ | $\frac{g^2}{\zeta'} \hat{a}^3 \ell_0^3 n = 1 - k^2 + (2k^2 - 1) \frac{E}{K}$ |
|------------------------------------------------------------------------|------------------------------------------------------------------------------|

|                                                                                                                                                                                                                                                                                                                             |                                                                                                                                                                         |
|-----------------------------------------------------------------------------------------------------------------------------------------------------------------------------------------------------------------------------------------------------------------------------------------------------------------------------|-------------------------------------------------------------------------------------------------------------------------------------------------------------------------|
| $z \sim z + 4K\alpha \quad \frac{\zeta' z}{\alpha \omega_0} \sim \frac{\zeta' z}{\alpha \omega_0} + \frac{2\pi}{\omega_0}$                                                                                                                                                                                                  | $T \sim T + \frac{2\pi}{\omega_0}$                                                                                                                                      |
| $ds^2 = t_{\text{Higgs}}^2 \hat{a}^2 \left( -dz^2 + \frac{1}{\epsilon^2} \hat{g}_{ij} dx^i dx^j \right)$ $= t_{\text{Higgs}}^2 \omega_0^2 \frac{\alpha^2 \hat{a}^2}{\zeta'^2} \left[ - \left( \frac{\zeta' dz}{\alpha \omega_0} \right)^2 + \frac{\zeta'^2 \hat{g}_{ij}}{\alpha^2 \omega_0^2 \epsilon^2} dx^i dx^j \right]$ | $ds^2 = \ell^2 a_\ell^2 \left( -dT^2 + g_{ij}^{(3)} dx^i dx^j \right)$ $= \ell_0^2 \omega_0^2 \frac{\hat{a}^2}{\zeta'^2} \left( -dT^2 + g_{ij}^{(3)} dx^i dx^j \right)$ |

## 11 Low density

G&R 8.113-4, DLMF 19.5.1-2, 19.12.1

$$\begin{aligned}
 k \rightarrow 0 \quad K(k) &= \frac{\pi}{2} \left( 1 + \frac{k^2}{4} + \frac{9k^4}{64} \right) + O(k^6) \\
 E(k) &= \frac{\pi}{2} \left( 1 - \frac{k^2}{4} - \frac{3k^4}{64} \right) + O(k^6) \\
 \frac{E}{K} &= 1 - \frac{k^2}{2} - \frac{k^4}{16} + O(k^6)
 \end{aligned} \tag{11.1}$$

$$\begin{aligned}
 C_1 &= \frac{1}{2}k^2(1 - k^2) \\
 C_2 &= 1 - 2k^2 \\
 C_3 &= k^2 - 1 + \frac{E}{K} = \frac{1}{2}k^2 \left( 1 - \frac{k^2}{8} \right) + O(k^6) \\
 \zeta' &= \frac{2\pi}{4K} = 1 - \frac{k^2}{4} + O(k^4) \\
 1 - k^2 + (2k^2 - 1)\frac{E}{K} &= 1 - k^2 + (2k^2 - 1) \left( 1 - \frac{k^2}{2} \right) + O(k^4) = \frac{3}{2}k^2 + O(k^4) \\
 C_4 &= \zeta' \left[ 1 - k^2 + (2k^2 - 1)\frac{E}{K} \right] = \frac{3}{2}k^2 + O(k^4) \\
 \hat{a}^2 &= \frac{4\lambda^2}{g^2}C_2 + \frac{3}{2}C_3 = \frac{4\lambda^2}{g^2} + O(k^2) \\
 \frac{\rho}{\rho_0} &= \frac{1}{\hat{a}^4} \left( \frac{3}{g^2}C_1 + \frac{9}{32\lambda^2}C_3^2 \right) = \left( \frac{g^2}{4\lambda^2} \right)^2 \frac{3}{g^2} \frac{1}{2}k^2 + O(k^4) \\
 &= \frac{3g^2}{32\lambda^4}k^2 + O(k^4) = 0.600 k^2 + O(k^4) \\
 \frac{p}{\rho_0} &= \frac{1}{\hat{a}^4} \left[ \frac{1}{g^2}(C_1 - C_2C_3) - \frac{9}{32\lambda^2}C_3^2 \right] \\
 C_1 - C_2C_3 &= \frac{1}{2}k^2 - \frac{1}{2}k^4 - (1 - 2k^2)\frac{1}{2}k^2 \left( 1 - \frac{k^2}{8} \right) = \frac{9}{16}k^4 \\
 \frac{p}{\rho_0} &= \left( \frac{g^2}{4\lambda^2} \right)^2 \left[ \frac{1}{g^2} \frac{9}{16}k^4 - \frac{9}{32\lambda^2} \frac{1}{4}k^4 \right] \\
 &= \frac{9g^4}{256\lambda^4} \left[ \frac{1}{g^2} - \frac{1}{8\lambda^2} \right] k^4 \\
 n &= \frac{1}{\ell_0^3} \frac{1}{\hat{a}^3} \frac{1}{g^2} C_4 = \frac{1}{\ell_0^3} \frac{g^3}{8\lambda^3} \frac{1}{g^2} \frac{3}{2}k^2 = \frac{1}{\ell_0^3} \frac{3g}{16\lambda^3} k^2
 \end{aligned} \tag{11.2}$$

**equation of state**

$$\begin{aligned} \frac{p}{\rho_0} &= \frac{9g^4}{256\lambda^4} \left[ \frac{1}{g^2} - \frac{1}{8\lambda^2} \right] k^4 = \frac{9g^4}{256\lambda^4} \left[ \frac{1}{g^2} - \frac{1}{8\lambda^2} \right] \left( \frac{32\lambda^4}{3g^2} \frac{\rho}{\rho_0} \right)^2 \\ &= 4\lambda^4 \left( \frac{1}{g^2} - \frac{1}{8\lambda^2} \right) \frac{\rho^2}{\rho_0^2} = \frac{1}{2} \frac{\lambda^2 (8\lambda^2 - g^2)}{g^2} \frac{\rho^2}{\rho_0^2} \end{aligned} \quad (11.3)$$

$$p = \frac{c_a}{2} \frac{\rho^2}{\rho_0} \quad c_a = \frac{\lambda^2 (8\lambda^2 - g^2)}{g^2} = 0.992 \quad (11.4)$$

**density of quanta**

$$n = \frac{1}{\ell_0^3} \frac{3g}{16\lambda^3} k^2 = \frac{1}{\ell_0^3} \frac{3g}{16\lambda^3} \frac{32\lambda^4}{3g^2} \frac{\rho}{\rho_0} = \frac{2\lambda}{g} \frac{\rho}{m_{\text{Higgs}}} = \frac{\rho}{m_W} \quad (11.5)$$

**present dark matter density and  $\langle k^2 \rangle_{\text{now}}$**

$$\begin{aligned} \rho_c &= \frac{3H_0^2}{8\pi G} = 8.53 \times 10^{-27} \text{kg/m}^3 \\ \langle \rho_{\text{CDM}} \rangle_{\text{now}} &= \Omega_{\text{CDM}} \rho_c = 0.27 \cdot 8.53 \times 10^{-27} \text{kg/m}^3 = 2.3 \times 10^{-27} \text{kg/m}^3 \\ \frac{\langle \rho_{\text{CDM}} \rangle_{\text{now}}}{\rho_0} &= 4.1 \times 10^{-56} \\ \langle k^2 \rangle_{\text{now}} &= \frac{32\lambda^4}{3g^2} \frac{\langle \rho_{\text{CDM}} \rangle_{\text{now}}}{\rho_0} = 1.67 \cdot 4.1 \times 10^{-56} = 7 \times 10^{-56} \end{aligned} \quad (11.6)$$

**TOV stability and central density**

From *Dark matter stars* [2], the maximum CGF star mass is

$$M_{\text{max}} = 9.145 \times 10^{-6} M_{\odot} \quad \rho_{\text{max}} = 0.799 \rho_0 \quad k_{\text{max}}^2 = 0.341 \quad (11.7)$$

The last two numbers are from the numerical solutions in Sagemath. The entire star is in the broken phase. The core is not in the low density regime.

The unit of mass in [2] is

$$m_b = (4\pi)^{-\frac{1}{2}} \frac{\ell}{G} = 2.94 \times 10^{-5} M_{\odot} \quad (11.8)$$

Here the unit of mass is

$$M_{\ell} = \frac{\ell}{G} = 1.04 \times 10^{-4} M_{\odot} \quad (11.9)$$

The TOV equation is exactly solvable with the low density equation of state

$$p = \frac{c_a}{2} \frac{\rho^2}{\rho_0} \quad c_a = 0.99248 \quad (11.10)$$

In the low density regime, [2, (5.1), (2.2)] give

$$\frac{M}{m_b} = \pi c_a^{3/2} \frac{\rho_{\text{central}}}{\rho_0} \quad (11.11)$$

which is

$$\frac{M}{M_\ell} = \frac{\pi^{1/2} c_a^{3/2}}{2} \frac{\rho_{\text{central}}}{\rho_0} = 0.87625 \frac{\rho_{\text{central}}}{\rho_0} \quad (11.12)$$

The parametrization by  $k^2$  is

$$\frac{\rho}{\rho_0} = \frac{3}{32} \frac{g^2}{\lambda^4} k^2 = 0.599698 k^2 \quad (11.13)$$

so

$$M = \frac{\pi^{1/2} c_a^{3/2}}{2} \frac{3}{32} \frac{g^2}{\lambda^4} M_\ell k_{\text{central}}^2 = 5.4782 \times 10^{-5} M_\odot k_{\text{central}}^2 \quad (11.14)$$

The microlensing limit  $M = 10^{-11} M_\odot$  corresponds to

$$k_{\text{central}}^2 = \frac{10^{-11} M_\odot}{5.4782 \times 10^{-5} M_\odot} = 1.825 \times 10^{-7} \quad (11.15)$$

## 12 Possibilities of detection and verification?

The metric in the rest frame is

$$ds^2 = \ell^2 g_{\mu\nu} dx^\mu dx^\nu = \ell^2 a_\ell(x)^2 \left[ -(dT)^2 + g_{ij}^{(3)}(x) dx^i dx^j \right] \quad (12.1)$$

In the low density regime  $a_\ell = 4\lambda^2/g^2$ .

$$ds^2 = \ell^2 \frac{4\lambda^2}{g^2} \left[ -(dT)^2 + g_{ij}^{(3)}(x) dx^i dx^j \right] \quad (12.2)$$

so proper time  $t$  is given by

$$t = \ell \frac{2\lambda}{g} T \quad (12.3)$$

The CGF oscillation period is

$$T \sim T + \frac{2\pi}{\omega_0} \quad (12.4)$$

so the period in proper time is

$$t \sim t + \frac{2\pi}{\omega_0} \ell \frac{2\lambda}{g} = t + 2\pi \ell_0 \frac{2\lambda}{g} = t + 2\pi \frac{\hbar}{m_{\text{Higgs}}} \frac{2\lambda}{g} = t + \frac{2\pi \hbar}{m_W} \quad (12.5)$$

The proper time frequency is

$$\omega_{\text{proper}} = \frac{m_W}{\hbar} \quad (12.6)$$

## References

- [1] D. Friedan, “A theory of the dark matter,” [arXiv:2203.12405 \[astro-ph.CO\]](#). March, 2022.
- [2] D. Friedan, “Dark matter stars,” [arXiv:2203.12181 \[astro-ph.CO\]](#). March, 2022.
